# Supplementary material for: Regret Lower Bounds for Decentralized Multi-Agent Stochastic Shortest Path Problems
Source: arXiv:2511.04594 source file (2025-12-13)
Supplement: Supplementary file 1 [file Lemma6.tex]

\nlowerbound*

% \textbf{Recall the Lemma  \ref{lemma:gen_co}.}  \textit{If $T \geq 2KV^*_1$, then, $\mathbb{E}_{\theta}[N^-] \geq KV^*_1/4$,  for any $\theta \in \Theta$.} 

\begin{proof}
Recall the capped process from Theorem \ref{thm:lower_bound} proof. If capped process finishes before $T$, then $N^-=N$. Else, number of visits to $goal$ state is less than $K$ due to which $N^- \geq T-K$. Therefore, we have
\begin{align}
    \mathbb{E}_{\theta, \pi}[N^-] \geq \mathbb{E}_{\theta, \pi}[\min\{T-K,N\}] \geq \mathbb{E}_{\theta, \pi}\left[ \sum_{i=1}^K\min\{T/K-1, N^{\pi}_k\} \right] \label{eqn:tknk}
\end{align}
In the above, $N^{\pi}_k$ is the random variable representing the length of episode $k$ when following $\pi$. Since $T\geq2KV^*_1,$ and $V^*_1\geq1$, we have $T/K-1>V^*_1$. Using this, from Equation \eqref{eqn:tknk}, we observe that the statement of lemma holds for any algorithm $\pi$ if $N^\pi_k \geq V^*_1$ with probability at least $ 1/4$. So, is suffices to prove that for any $\pi$, the probability that $N^\pi_k \geq V^*_1$ is at least $1/4$.

For this first observe the following lemma (proof in Appendix \ref{proof:lemma_episodelength})
\begin{restatable*}{lem}{probnk}
\label{lemma:episodelength}
    Let's define the notation $\mathbb{P}[N^{\pi}_k(\tb{\ti{s}}) \geq x]$ as the probability that starting at state $\tb{\ti{s}} \in \mathcal{S}$ and following the algorithm $\pi$, the number of time steps required to reach global goal in episode $k$ (i.e., $ N^{\pi}_k(\tb{\ti{s}}))$ is more than or equal to $x$ for any $x \in \mathbb{R}^+$.  Additionally, define $\mathbb{P}[N_k^{\pi} \geq x] := \mathbb{P}[N_k^{\pi}(\tb{\ti{s}}_{\init}) \geq x] $, which is the probability when starting from the initial state $\tb{\ti{s}}_{\init} $.
    Let $ \pi^* $ be the optimal policy that chooses the action $ \tb{\ti{a}}^* = \tb{\ti{a}}_\theta $ in every state $ \tb{\ti{s}} \in \mathcal{S} $, as defined in Theorem~\ref{thm:all_in_one}.

    Then, for any algorithm $ \pi $, for all $ x \in \mathbb{R}^+ $, $ k \in \mathbb{N} $, and any state $ \tb{\ti{s}} \in \mathcal{S}_r $ with $ r \in [n] $, we have
\begin{align}
    \mathbb{P}[N_k^{\pi}(\tb{\ti{s}}) \geq x] \geq  \mathbb{P}[N_k^{\pi^*}(\tb{\ti{s}}) \geq x] = \mathbb{P}[N_k^{\pi^*}(r) \geq x]  \geq \mathbb{P}[N_k^{\pi^*}(\tb{\ti{s}}') \geq x]
\end{align}
where $\tb{\ti{s}}' \in \mathcal{S}(\tb{\ti{s}})$ with equalities holding at $\pi = \pi^*$  and $r'=r $ (i.e., $\tb{\ti{s}}'=\tb{\ti{s}}$) respectively. The equality in the middle indicates that under $\pi^*$, $\mathbb{P}[N_k^{\pi^*}(\tb{\ti{s}}) \geq x]$ stays constant for all $\tb{\ti{s}} \in \mathcal{S}_r$, for every $r \in [n]$, depending only on $r$.
\end{restatable*}

% Lemma \ref{lemma:episodelength}, \pt{This is again using lemma 5, need to write the proof of lemma 5 before lemma 6, then.} \textcolor{blue}{yes} 

% \textcolor{blue}{need to fix the lemma labels here }

Using above lemma, for $\tb{\ti{s}} = \tb{\ti{s}}_{\init}, \tb{\ti{s}}' = \tilde{\tb{\ti{s}}}$  for some $\tilde{\tb{\ti{s}}} \in \mathcal{S}_1,$ we have 
\begin{align}
    \mathbb{P}[N^{\pi}_k(\tb{\ti{s}}_{\init}) \geq V^*_1] 
    &\geq 
    \mathbb{P}[N_k^{\pi^*}(\tb{\ti{s}}_{\init}) \geq V^*_1]  
    \\
    &\geq \mathbb{P}[N_k^{\pi^*}(\tilde{\tb{\ti{s}}}) \geq V^*_1] 
    \\
    &= (1-\mathbb{P}(\tb{\ti{g}}|\tilde{\tb{\ti{s}}},\tb{\ti{a}}^*))^{\lfloor V^*_1 \rfloor  } \label{eqn:lastthird}
    \\
    &\geq (1-\mathbb{P}(\tb{\ti{g}}|\tilde{\tb{\ti{s}}},\tb{\ti{a}}^*))^{ V^*_1 }  \label{eqn:lastsecond}
    \\
    &\geq 1/4
\end{align}
Equation \eqref{eqn:lastthird} follows as the event is a Bernoulli trial (either next state is same as $\tilde{\tb{\ti{s}}}$ or $\tb{\ti{g}}$). Further, the last inequality follows from the fact that $V^*_1 = 1/p^*(goal|\tilde{\tb{\ti{s}}}_1, \tb{\ti{a}}^*)$ (see proof of Theorem \ref{thm:all_in_one}) and for $x>2$, $(1-1/x)^x \geq 1/4$. 

Note that $V^*_1 = \frac{2n}{n-1+2(\delta+\Delta)} > 2$ since 
\begin{align}
    \frac{1}{V^*_1} & = \frac{n-1}{2n} + \frac{2(\delta+\Delta)}{2n} 
    \\
    & < \frac{n-1}{2n} + \frac{2(\delta+2^{-n}.\frac{1-2\delta}{1+n+n^2})}{2n} 
    \\
    & < \frac{n-1}{2n} + \frac{2(\delta+\frac{1-2\delta}{6})}{2n} 
    \\
    &= \frac{n-1}{2n} + \frac{(\frac{1+4\delta}{3})}{2n} 
    \\
    & < 1/2
\end{align}
Above, the first inequality arises because $\Delta < \frac{1-2\delta}{1+n+n^2}$ for our instances, the second inequality holds because $n \geq 1$ and the final step is due to $\delta < 1/2$.
\end{proof}
