# Supplementary material for: Regret Lower Bounds for Decentralized Multi-Agent Stochastic Shortest Path Problems
Source: arXiv:2511.04594 source file (2025-12-13)
Supplement: Supplementary file 2 [file Lemma8.tex]

\subsection{Proof of Lemma \ref{lemma:episodelength}}
\label{proof:lemma_episodelength}

\probnk

\begin{proof}
 
We will prove this by induction over $r$ (\emph{type} of a state).

\tb{Base Case:} For $r=1$

Consider any $\tb{\ti{s}} \in \mathcal{S}_1$. For any $x \in \mathbb{R}^+$, we have that 
\begin{align}
 \mathbb{P}[N_k^{\pi}(\tb{\ti{s}}) \geq x] = (1-\mathbb{P}(\tb{\ti{g}}|\tb{\ti{s}},\pi(\tb{\ti{s}})))^{\lceil x\rceil-1}
\end{align}

Using Lemma \ref{lemma:general_tp}, 
the above is minimized when $\pi(\tb{\ti{s}}) = \tb{\ti{a}}^*$. The above arguments hold for any $\tb{\ti{s}} \in \mathcal{S}_1$ and $x \in \mathbb{R}^+$.
Hence the equality holds for all $\tb{\ti{s}} \in \mathcal{S}_1$ for any $x \in \mathbb{R}^+$ at $\pi=\pi^*$. 
Hence,
\begin{align}\label{eqn:prob_n}
 \mathbb{P}[N_k^{\pi}(\tb{\ti{s}}) \geq x] = (1-\mathbb{P}(\tb{\ti{g}}|\tb{\ti{s}},\pi(\tb{\ti{s}})))^{\lceil x\rceil-1} \geq (1-\mathbb{P}(\tb{\ti{g}}|\tb{\ti{s}},\pi^*(\tb{\ti{s}})))^{\lceil x\rceil -1}
\end{align}
Recall that for the same action $\tb{\ti{a}}^*$ at any $\tb{\ti{s}} \in \mathcal{S}_1$, $\mathbb{P}(\tb{\ti{g}}|\tb{\ti{s}},\tb{\ti{a}}^*)$ remains the same (Corollary \ref{corollary:p_star}). Hence, we further have, 
\begin{align}
    \mathbb{P}[N_k^{\pi}(\tb{\ti{s}}) \geq x] &= (1-\mathbb{P}(\tb{\ti{g}}|\tb{\ti{s}},\pi(\tb{\ti{s}})))^{\lceil x \rceil-1} 
    \\
    & \geq (1-\mathbb{P}(\tb{\ti{g}}|\tb{\ti{s}},\pi^*(\tb{\ti{s}})))^{\lceil x \rceil -1} 
    \\
    &= \mathbb{P}[N_k^{\pi^*}(\tb{\ti{s}}) \geq x]
    \\
    & = \mathbb{P}[N_k^{\pi^*}(r=1) \geq x] 
\end{align}

Now, for the base case, the last inequality in the Lemma statement remains to be shown.

For any $\tb{\ti{s}}\in \mathcal{S}_1$, the only two possibilities for next state $\tb{\ti{s}}'$ are $\tb{\ti{s}}$ and $\tb{\ti{g}}$. 
Clearly, for $\tb{\ti{s}}=\tb{\ti{s}}'$ the equality holds while for $\tb{\ti{s}}' = \tb{\ti{g}}$, we have that $\mathbb{P}[N_k^{\pi^*}(\tb{\ti{s}}') \geq x] = 0$. Hence, from the above inequality we have that
\begin{align}
    \mathbb{P}[N_k^{\pi}(\tb{\ti{s}}) \geq x] 
    &\geq \mathbb{P}[N_k^{\pi^*}(r=1) \geq x] 
    \\
    &\geq  \mathbb{P}[N_k^{\pi^*}(\tb{\ti{s}}') \geq x] 
\end{align}

From the above, we have that for any $x \in \mathbb{R}^+$, for any $\pi$, for any $\tb{\ti{s}} \in \mathcal{S}_1$ and $\tb{\ti{s}}' \in \cup_{r' \in \{0,1\}} \mathcal{S}_{r'}(\tb{\ti{s}})$, we have that
\begin{align}
    \mathbb{P}[N_k^{\pi}(\tb{\ti{s}}) \geq x]  \geq  \mathbb{P}[N_k^{\pi^*}(\tb{\ti{s}}) \geq x] = \mathbb{P}[N_k^{\pi^*}(r=1) \geq x] \geq  \mathbb{P}[N_k^{\pi^*}(\tb{\ti{s}}') \geq x] 
\end{align}
where in the first inequality, equality holds for all $x \in \mathbb{R}^+$ and $\tb{\ti{s}} \in \mathcal{S}_1$ if $\pi = \pi^*$, the middle equality means that the probability is same for all $\tb{\ti{s}} \in \mathcal{S}_1$ and in the last inequality, equality holds when $\tb{\ti{s}}' = \tb{\ti{s}}$.

This completes the proof for the base case.

\tb{Inductive Step:} Assume the above holds for $m = 1, 2,\dots,r$ i.e., for all $m \in [r]$ it holds that for any $x \in \mathbb{R}^+$, for any $\tb{\ti{s}} \in \mathcal{S}_m$, for any algorithm $\pi$, for our instances, 
\begin{align}
\mathbb{P}[N_k^{\pi}(\tb{\ti{s}}) \geq x] \geq \mathbb{P}[N_k^{\pi^*}(\tb{\ti{s}}) \geq x]=\mathbb{P}[N_k^{\pi^*}(m) \geq x]\geq \mathbb{P}[N_k^{\pi^*}(\tb{\ti{s}}')  \geq x]  
\end{align}
where $\pi^*$ is the policy taking action $\tb{\ti{a}}^*=\tb{\ti{a}}_{\theta}$ at all states and $\tb{\ti{s}}' \in \cup_{m' \in \{0\} \cup [m] }\mathcal{S}_{m'}(\tb{\ti{s}}) = \mathcal{S}(\tb{\ti{s}})$. 
Further, in the first inequality, equality holds for all $x \in \mathbb{R}^+$ and $\tb{\ti{s}} \in \mathcal{S}_m$ when $\pi =\pi^*$ and the middle equality implies that the probability is same for all states of same \emph{type} 
% \pt{type is always denoted by, r not by state itself?} 
i.e., $\tb{\ti{s}} \in \mathcal{S}_m$ and in the last inequality, the equality holds only when $\tb{\ti{s}}' = \tb{\ti{s}}$.  

Assuming the above, we need to show that the same holds for any state of type $r+1$, i.e., for any state $\tb{\ti{s}} \in \mathcal{S}_{r+1}$. To this end consider any $x \in \mathbb{R}^+$ and any $\tb{\ti{s}} \in \mathcal{S}_{r+1}$. Then, we have 
\begin{align}
    &\mathbb{P}[N_k^{\pi}(\tb{\ti{s}}) \geq x] \nonumber
    \\
    &= \sum_{r'=0}^{r+1} ~ \sum_{\tb{\ti{s}}' \in \mathcal{S}_{r'}(\tb{\ti{s}})} \mathbb{P}(\tb{\ti{s}}'|\tb{\ti{s}},\pi(\tb{\ti{s}})) \cdot \mathbb{P}[N_k^{\pi}(\tb{\ti{s}}') \geq x-1] 
    \\
    &= \mathbb{P}(\tb{\ti{s}}|\tb{\ti{s}},\pi(\tb{\ti{s}})) \cdot \mathbb{P}[N_k^{\pi}(\tb{\ti{s}})  \geq x-1] + \sum_{r' = 0}^{r} \sum_{\tb{\ti{s}}' \in \mathcal{S}_{r'}(\tb{\ti{s}})}  \mathbb{P}(\tb{\ti{s}}'|\tb{\ti{s}},\pi(\tb{\ti{s}})) \cdot \mathbb{P}[N_k^{\pi}(\tb{\ti{s}}') \geq x-1]  
\end{align}
The first equality holds by 1-time step decomposition of the event $N^\pi_k(\tb{\ti{s}}') \geq x$. 
If $x \leq 1$, then for any $\pi$,  $\mathbb{P}[N_k^{\pi} \geq x] = 1$ for all $\tb{\ti{s}} \neq \tb{\ti{g}}$. This is because there will at least be 1 time step to reach $\tb{\ti{g}}$ from any non-goal state.
% \pt{because of this reason, we need to use $\pi$ in the notations.}

However, in general, we have the following
\begin{align}
    & \mathbb{P}[N_k^{\pi}(\tb{\ti{s}}) \geq x]  \nonumber
    \\
    &=  \mathbb{P}(\tb{\ti{s}}|\tb{\ti{s}},\pi(\tb{\ti{s}})) \mathbb{P}[N_k^{\pi}(\tb{\ti{s}}) \geq x-1] + \sum_{r' =0}^r \sum_{\tb{\ti{s}}' \in \mathcal{S}_{r'}(\tb{\ti{s}})}  \mathbb{P}(\tb{\ti{s}}'|\tb{\ti{s}},\pi(\tb{\ti{s}})) \mathbb{P}[N_k^{\pi}(\tb{\ti{s}}') \geq x-1] 
    \\
    &\geq \mathbb{P}(\tb{\ti{s}}|\tb{\ti{s}},\pi(\tb{\ti{s}})) \mathbb{P}[N_k^{\pi}(\tb{\ti{s}}) \geq x-1] + \sum_{r' = 0}^r \sum_{\tb{\ti{s}}' \in \mathcal{S}_{r'}(\tb{\ti{s}})}  \mathbb{P}(\tb{\ti{s}}'|\tb{\ti{s}},\pi(\tb{\ti{s}})) \mathbb{P}[N_k^{\pi^*}(r') \geq x-1] 
\end{align}
The above follows from induction assumption.
Thus, we have that
\begin{align}
    &\mathbb{P}[N_k^{\pi}(\tb{\ti{s}}) \geq x]  \nonumber
    \\   
    &\geq  \mathbb{P}(\tb{\ti{s}}|\tb{\ti{s}},\pi(\tb{\ti{s}})) \cdot \mathbb{P}[N_k^{\pi}(\tb{\ti{s}}) \geq x-1] + \sum_{r' =0}^{r} \mathbb{P}[N_k^{\pi^*}(r') \geq x-1] \sum_{\tb{\ti{s}}' \in \mathcal{S}_{r'}(\tb{\ti{s}})}  \mathbb{P}(\tb{\ti{s}}'|\tb{\ti{s}},\pi(\tb{\ti{s}})) 
    \\
    &= \mathbb{P}(\tb{\ti{s}}|\tb{\ti{s}},\pi(\tb{\ti{s}})) \cdot \mathbb{P}[N_k^{\pi}(\tb{\ti{s}}) \geq x-1] +  \sum_{r' =0}^r \mathbb{P}[N_k^{\pi^*}(r')  \geq x-1] \nonumber
    \\ 
    & \quad \times \sum_{\tb{\ti{s}}' \in \mathcal{S}_{r'}(\tb{\ti{s}})} \Bigg[ \frac{r' + (r+1-2r')\delta}{n \cdot 2^r} +   \frac{n-r-1}{n2^{r+1}} +    \frac{\Delta}{n}  (r+1-2r') \nonumber 
    \\
    &\quad + \frac{2 \Delta}{n(d-1)} \sum_{p=1}^{d-1} \left(  \sum_{i \in \mathcal{I} \cap \mathcal{T'}} \mathbbm{1}\{\sgn(a_{i,p}) \neq \sgn(\theta_{i,p})\}   -\sum_{t \in \mathcal{T}}  \mathbbm{1}\{\sgn(a_{t,p}) \neq \sgn(\theta_{t,p})\} \right)  \Bigg]
    \\
    &= \mathbb{P}(\tb{\ti{s}}|\tb{\ti{s}},\pi(\tb{\ti{s}})) \cdot \mathbb{P}[N_k^{\pi}(\tb{\ti{s}})  \geq x-1] \nonumber
    \\ 
    &\quad + \sum_{r' =0}^r \mathbb{P}[N_k^{\pi^*} (r') \geq x-1] \cdot  \sum_{\tb{\ti{s}}' \in \mathcal{S}_{r'}(\tb{\ti{s}})} \left( \frac{r' + (r+1-2r')\delta}{n \cdot 2^r} +   \frac{n-r-1}{n2^{r+1}}   +   \frac{\Delta}{n}  (r+1-2r') \right) \nonumber
    \\ 
    &\quad + \sum_{r' =0}^r \mathbb{P}[N_k^{\pi^*} (r') \geq x-1]  \nonumber
    \\
    &\quad  \times \sum_{\tb{\ti{s}}' \in \mathcal{S}_{r'}(\tb{\ti{s}})}  \frac{2 \Delta}{n(d-1)} \sum_{p=1}^{d-1} \left(  \sum_{i \in \mathcal{I} \cap \mathcal{T'}}\mathbbm{1}\{\sgn(a_{i,p}) \neq \sgn(\theta_{i,p})\}   -\sum_{t \in \mathcal{T}} \mathbbm{1}\{\sgn(a_{t,p}) \neq \sgn(\theta_{t,p})\} \right)  
\end{align}
In the first term, we observe that the term inside the inner summation over $s' \in \mathcal{S}_{r'}(\tb{\ti{s}}')$, the terms inside that summation do not depend on which $\tb{\ti{s}}'$ is being considered for a fixed $r'$ and $\tb{\ti{s}}$ and are the same. 
Hence, the whole summation simplifies to the product of this term and the cardinality of that set which is $\binom{r+1}{r'}$. Also, we realize that for the second term for any agent the coefficient of the indicator is $+1$ if he stays at node $s$ itself while it is $-1$ when he transits to node $g$. Hence we can simplify the above by rearranging summations and using the fact that the probability terms vanish for state of \emph{type} 0, namely $\tb{\ti{g}}$.
\begin{align}
    &\mathbb{P}[N_k^{\pi}(\tb{\ti{s}}) \geq x]  \nonumber
    \\   
    &\geq \mathbb{P}(\tb{\ti{s}}|\tb{\ti{s}},\pi(\tb{\ti{s}})) \cdot \mathbb{P}[N_k^{\pi}(\tb{\ti{s}}) \geq x-1] \nonumber
    \\ 
    &\quad + \sum_{r'=1}^r \binom{r+1}{r'} \mathbb{P}[N_k^{\pi^*}(r') \geq x-1] \cdot   \left( \frac{r' + (r+1-2r')\delta}{n \cdot 2^r} +   \frac{n-r-1}{n2^{r+1}}   + \frac{\Delta}{n}  (r+1-2r') \right) \nonumber
    \\ 
    &\quad + \frac{2 \Delta}{n(d-1)} \times \sum_{p=1}^{d-1} \sum_{r' \in  [r]} \mathbb{P}[N_k^{\pi^*}(r') \geq x-1] \nonumber
    \\
    &\quad \times \sum_{\tb{\ti{s}}' \in \mathcal{S}_{r'}(\tb{\ti{s}})} \sum_{i \in \mathcal{I}}      \left( \mathbbm{1}\{i \in \mathcal{I} \cap \mathcal{T'}\}.   - \mathbbm{1}\{i \in \mathcal{T}\} \right) \cdot \mathbbm{1}\{\sgn(a_{i,p}) \neq \sgn(\theta_{i,p})\} 
    \\
    & = \mathbb{P}(\tb{\ti{s}}|\tb{\ti{s}},\pi(\tb{\ti{s}})) \cdot \mathbb{P}[N_k^{\pi}(\tb{\ti{s}}) \geq x-1] \nonumber
    \\ 
    & \quad + \sum_{r'=1}^r \binom{r+1}{r'} \mathbb{P}[N_k^{\pi^*}(r') \geq x-1] \cdot  \left( \frac{r' + (r+1-2r')\delta}{n \cdot 2^r} +   \frac{n-r-1}{n2^{r+1}}   +    \frac{\Delta}{n}  (r+1-2r') \right) \nonumber
    \\ 
    &\quad + \frac{2 \Delta}{n(d-1)} \sum_{p=1}^{d-1} \sum_{r'=1}^r \mathbb{P}[N_k^{\pi^*}(r') \geq x-1]  \sum_{i \in \mathcal{I}}      \left( \binom{r}{r'-1} -  \binom{r}{r'} \right) \cdot  \mathbbm{1}\{\sgn(a_{i,p}) \neq \sgn(\theta_{i,p})\}
\end{align}
The last step follows by taking the summation over $s'$ inside and observing that from any fixed $\tb{\ti{s}}$ of \emph{type} $r$, the number of states of \emph{type} $r'$ reachable from $\tb{\ti{s}}$ in which any agent at node $s$ stays at node $s$ is $\binom{r}{r'-1}$ and those in which the agent transits to node $g$ is $\binom{r}{r'}$. Thus, we have
\begin{align}
    &\mathbb{P}[N_k^{\pi}(\tb{\ti{s}}) \geq x]  \nonumber
    \\  
    &\geq \mathbb{P}(\tb{\ti{s}}|\tb{\ti{s}},\pi(\tb{\ti{s}})) \cdot \mathbb{P}[N_k^{\pi}(\tb{\ti{s}}) \geq x-1] \nonumber
    \\ 
    & \quad + \sum_{r'=1}^r \binom{r+1}{r'} \mathbb{P}[N_k^{\pi^*} (r')\geq x-1] \cdot  \left( \frac{r' + (r+1-2r')\delta}{n \cdot 2^r} +   \frac{n-r-1}{n2^{r+1}}   +  \frac{\Delta}{n}  (r+1-2r') \right) \nonumber
    \\ 
    &\quad + \frac{2 \Delta}{n(d-1)} \sum_{p=1}^{d-1} \sum_{r'=1}^r \sum_{i \in \mathcal{I}} \mathbb{P}[N_k^{\pi^*}(r') \geq x-1]         \left(  \binom{r}{r'-1} -  \binom{r}{r'}  \right) \mathbbm{1}\{\sgn(a_{i,p}) \neq \sgn(\theta_{i,p})\}
    \\
    & = \mathbb{P}(\tb{\ti{s}}|\tb{\ti{s}},\pi(\tb{\ti{s}})) \cdot \mathbb{P}[N_k^{\pi}(\tb{\ti{s}}) \geq x-1] \nonumber
    \\ 
    & \quad + \sum_{r'=1}^r \binom{r+1}{r'} \mathbb{P}[N_k^{\pi^*}(r') \geq x-1] \cdot \left( \frac{r' + (r+1-2r')\delta}{n \cdot 2^r} +   \frac{n-r-1}{n2^{r+1}}   +    \frac{\Delta}{n}  (r+1-2r') \right)  \nonumber
    \\ 
    &\quad + \frac{\Delta}{n(d-1)} \sum_{p=1}^{d-1} \sum_{i \in \mathcal{I}} \sum_{r'=1}^r \Bigg[  \mathbb{P}[N_k^{\pi^*}(r') \geq x-1]  \left( \binom{r}{r'-1} -  \binom{r}{r'} \right) \mathbbm{1}\{\sgn(a_{i,p}) \neq \sgn(\theta_{i,p})\} \nonumber
    \\
    &\quad + \mathbb{P}[N_k^{\pi^*}(r+1-r')  \geq x-1]   \left(  \binom{r}{r-r'} -  \binom{r}{r+1-r'} \right) \cdot \mathbbm{1}\{\sgn(a_{i,p}) \neq \sgn(\theta_{i,p})\} \Bigg]   
\end{align}
In the last step we use the following: for any function $f$, and $m \in \mathbb{N}$ we have, $2\cdot\sum_{a\in[m]}f(a) = \sum_{a\in[m]}f(a) + \sum_{a\in[m]} f(m+1-a)$.
% } \textcolor{blue}{not clear why $2 \Delta$ term gives one $\Delta
% $ term and an extra term in Eq 244, which means that this term is $\Delta$ term}
The above equation can be simplified as follows
\begin{align}
    &\mathbb{P}[N_k^{\pi}(\tb{\ti{s}}) \geq x] \nonumber
    \\    
    &= \mathbb{P}(\tb{\ti{s}}|\tb{\ti{s}},\pi(\tb{\ti{s}})) \cdot \mathbb{P}[N_k^{\pi}(\tb{\ti{s}}) \geq x-1] \nonumber
    \\ 
    &\quad + \sum_{r'=1}^r \binom{r+1}{r'} \mathbb{P}[N_k^{\pi^*}(r') \geq x-1] \cdot \left( \frac{r' + (r+1-2r')\delta}{n \cdot 2^r} +   \frac{n-r-1}{n2^{r+1}}   +    \frac{\Delta}{n}  (r+1-2r') \right)  \nonumber
    \\ 
    &\quad + \frac{\Delta}{n(d-1)} \sum_{p=1}^{d-1}  \sum_{i \in \mathcal{I}} \sum_{r'=1}^r \Bigg[ \mathbb{P}[N_k^{\pi^*} (r') \geq x-1] \left( \binom{r}{r'-1} -  \binom{r}{r'} \right) \mathbbm{1}\{\sgn(a_{i,p}) \neq \sgn(\theta_{i,p})\}   \nonumber
    \\
    &\quad + \mathbb{P}[N_k^{\pi^*}(r+1-r') \geq x-1]  \left( \binom{r}{r'} -  \binom{r}{r'-1} \right) \mathbbm{1}\{\sgn(a_{i,p}) \neq \sgn(\theta_{i,p})\} \Bigg] 
    \\
    &= \mathbb{P}(\tb{\ti{s}}|\tb{\ti{s}},\pi(\tb{\ti{s}})) \cdot \mathbb{P}[N_k^{\pi}(\tb{\ti{s}}) \geq x-1] \nonumber
    \\
    &\quad + \sum_{r'=1}^r \binom{r+1}{r'} \mathbb{P}[N_k^{\pi^*}(r') \geq x-1] \cdot  \left( \frac{r' + (r+1-2r')\delta}{n \cdot 2^r} +   \frac{n-r-1}{n2^{r+1}}   +    \frac{\Delta}{n}  (r+1-2r') \right)  \nonumber
    \\
    &\quad + \frac{\Delta}{n(d-1)} \sum_{p=1}^{d-1}  \sum_{i \in \mathcal{I}} \sum_{r'=1}^r \Bigg[ \left( \binom{r}{r'-1} -  \binom{r}{r'} \right) \times \nonumber
    \\
    & \quad \hspace{1.5 cm} \left( \mathbb{P}[N_k^{\pi^*} (r') \geq x-1] - \mathbb{P}[N_k^{\pi^*} (r+1-r') \geq x-1] \right) \cdot \mathbbm{1}\{\sgn(a_{i,p}) \neq \sgn(\theta_{i,p})\}  \Bigg]
\end{align}
Notice that for $r' \leq  (r+1)/2$ the binomial difference $\binom{r}{r'-1} - \binom{r}{r'} \leq 0$. Moreover, the probability difference $\mathbb{P}[N_k^{\pi^*}(r') \geq x-1] - \mathbb{P}[N_k^{\pi^*}(r+1-r') \geq x-1] \leq  0$ due to induction assumption, hence the product in the last term of above equation is non-negative. Similar argument holds when $r'\geq (r+1)/2$. 

Overall we can observe that the only terms dependent on action have non-negative coefficients for the sign matching indicator. Hence the overall summation will be minimum when this term will be minimum which happens at $\tb{\ti{a}} = \tb{\ti{a}}^*=\tb{\ti{a}}_{\theta}$. Thus, we have
\begin{align}
    &\mathbb{P}[N_k^{\pi}(\tb{\ti{s}}) \geq x] \nonumber
    \\
    & \geq   \mathbb{P}(\tb{\ti{s}}|\tb{\ti{s}},\pi(\tb{\ti{s}})) \cdot \mathbb{P}[N_k^{\pi}(\tb{\ti{s}}) \geq x-1] \nonumber
    \\ 
    & \quad +\sum_{r'=1}^r \binom{r+1}{r'} \mathbb{P}[N_k^{\pi^*}(r') \geq x-1] \cdot  \left( \frac{r' + (r+1-2r')\delta}{n \cdot 2^r} +   \frac{n-r-1}{n2^{r+1}}        +    \frac{\Delta}{n}  (r+1-2r') \right)  \label{pnpi}
\end{align}
Also for the optimal policy $\pi^*$, we have
\begin{align}
    & \mathbb{P}[N_k^{\pi^*}(\tb{\ti{s}}) \geq x] 
    \\
    & =  \mathbb{P}(\tb{\ti{s}}|\tb{\ti{s}},\pi^*(\tb{\ti{s}})) \cdot \mathbb{P}[N_k^{\pi^*}(\tb{\ti{s}}) \geq x-1] \nonumber \\
    &\quad+  \sum_{r'=1}^r \binom{r+1}{r'} \mathbb{P}[N_k^{\pi^*}(r') \geq x-1] \cdot \left( \frac{r' + (r+1-2r')\delta}{n \cdot 2^r} + \frac{n-r-1}{n2^{r+1}}        +    \frac{\Delta}{n}  (r+1-2r') \right)
\label{eqn:p_npi*_k}
\end{align}
Subtracting the above two equations \eqref{pnpi} and \eqref{eqn:p_npi*_k} we get
\begin{align}
    &\mathbb{P}[N_k^{\pi}(\tb{\ti{s}})\geq x] - \mathbb{P}[N_k^{\pi^*}(\tb{\ti{s}})\geq x] \nonumber
    \\ 
    &\geq \mathbb{P}(\tb{\ti{s}}|\tb{\ti{s}},\pi(\tb{\ti{s}})) \mathbb{P}[N_k^{\pi}(\tb{\ti{s}}) \geq x-1] - \mathbb{P}(\tb{\ti{s}}|\tb{\ti{s}},\pi^*(\tb{\ti{s}})) \mathbb{P}[N_k^{\pi^*}(\tb{\ti{s}}) \geq x-1] \\ 
    &\geq \mathbb{P}(\tb{\ti{s}}|\tb{\ti{s}},\pi^*(\tb{\ti{s}})) \mathbb{P}[N_k^{\pi}(\tb{\ti{s}}) \geq x-1] - \mathbb{P}(\tb{\ti{s}}|\tb{\ti{s}},\pi^*(\tb{\ti{s}})) \mathbb{P}[N_k^{\pi^*} (\tb{\ti{s}}) \geq x-1]\\ 
    &= \mathbb{P}(\tb{\ti{s}}|\tb{\ti{s}},\pi^*(\tb{\ti{s}})) (\mathbb{P}[N_k^{\pi}(\tb{\ti{s}}) \geq x-1] - \mathbb{P}[N_k^{\pi^*}(\tb{\ti{s}})) \geq x-1]
\end{align}
where the last second step follows from Corollary \ref{corollary:ps_s}.

By recursion over $x$ we have
\begin{align}\label{eqn:pnxnx}
    \mathbb{P}[N_k^{\pi}(\tb{\ti{s}})\geq x] - \mathbb{P}[N_k^{\pi^*}(\tb{\ti{s}}) \geq x] 
    & \geq \mathbb{P}(\tb{\ti{s}}|\tb{\ti{s}},\pi^*(\tb{\ti{s}}))^{\lfloor x \rfloor} \{\mathbb{P}[N_k^{\pi}(\tb{\ti{s}}) \geq x-\lfloor x \rfloor] - \mathbb{P}[N_k^{\pi^*}(\tb{\ti{s}}) \geq x-\lfloor x \rfloor]\}  \nonumber
    \\
    &= \mathbb{P}(\tb{\ti{s}}|\tb{\ti{s}},\pi^*(\tb{\ti{s}}))^{\lfloor x \rfloor} (1- 1) 
    \\
    &= 0
\end{align}
In the last second step, we use the fact that $x-[x]$ is a fractional value or equal to $0$ for any $x \in \mathbb{R}^+$ hence for any $\tb{\ti{s}} \neq \tb{\ti{g}},$ certainly (with probability 1), at least one time step is required to reach reach $\tb{\ti{g}}$. Thus,
\begin{align}
    \mathbb{P}[N_k^{\pi}(\tb{\ti{s}}) \geq x] \geq \mathbb{P}[N_k^{\pi^*}(\tb{\ti{s}})\geq x] 
\end{align}
Clearly, equality holds at $\pi = \pi^*$. 
Recall from Equation \eqref{eqn:p_npi*_k} for any $\tb{\ti{s}} \in \mathcal{S}_{r+1}$ we have
\begin{align}
    &\mathbb{P}[N_k^{\pi^*}(\tb{\ti{s}}) 
    \geq x]\nonumber
    \\
    & = \mathbb{P}(\tb{\ti{s}}|\tb{\ti{s}},\pi^*(\tb{\ti{s}})) \mathbb{P}[N_k^{\pi^*}(\tb{\ti{s}})  \geq x-1] \label{eqn:prob_nxs}
    \\ 
    & \quad + \sum_{r'=1}^r \binom{r+1}{r'} \mathbb{P}[N_k^{\pi^*}(r') \geq x-1] \cdot \left( \frac{r' + (r+1-2r')\delta}{n \cdot 2^r} +   \frac{n-r-1}{n2^{r+1}}   +   \frac{\Delta}{n}  (r+1-2r') \right) \label{eqn:pneq}
\end{align}
From the probability expression one can verify that in the first term, $\mathbb{P}(\tb{\ti{s}}|\tb{\ti{s}},\pi^*(\tb{\ti{s}}))$ only depends on $r$. The second term is independent of $\tb{\ti{s}} \in \mathcal{S}_{r+1}$ due to induction hypothesis.

Thus, the only term in the above expression that may differ due to $\tb{\ti{s}}$ is $\mathbb{P}[N_k^{\pi^*}(\tb{\ti{s}}) \geq x-1]$.
We show below that this is the same for all $\tb{\ti{s}} \in \mathcal{S}_{r+1}$.  To this end, we apply the induction on $x$ itself.

% This can be dealt with by induction on $x$ itself.  \\

For the base case $b = x-\lfloor x \rfloor$, we have $\mathbb{P}[N_k^{\pi^*}(\tb{\ti{s}}) \geq m]=1$ for any $\tb{\ti{s}} \in \mathcal{S}_{r+1}$. Hence, the claim holds for the base case.

Assuming the claim holds for $ x - \lfloor x \rfloor,  x - \lfloor x \rfloor+1,  x - \lfloor x \rfloor+2, \dots,  x - \lfloor x \rfloor+q $, we will show that it holds for $b =  x - \lfloor x \rfloor + q+1$. To this end, note that for any $\tb{\ti{s}} \in \mathcal{S}_{r+1}$ we can write the following  
\begin{align}
    &\mathbb{P}[N_k^{\pi^*}(\tb{\ti{s}}) \geq b ] \nonumber
    \\
    &=\mathbb{P}(\tb{\ti{s}}|\tb{\ti{s}},\pi^*(\tb{\ti{s}})) \mathbb{P}[N_k^{\pi^*}(\tb{\ti{s}}) \geq b-1]  \nonumber
    \\
    & \quad +  \sum_{r'=1}^r \binom{r+1}{r'} \mathbb{P}[N_k^{\pi^*}(r') \geq b-1] \cdot \left( \frac{r' + (r+1-2r')\delta}{n \cdot 2^r} +   \frac{n-r-1}{n2^{r+1}}        +    \frac{\Delta}{n}  (r+1-2r') \right)  
\end{align}
From induction hypothesis and Corollary \ref{corollary:p_star}, the RHS doesn't depend on chosen $\tb{\ti{s}} \in \mathcal{S}_r$. 
Thus, the claim holds for $ b = x - \lfloor x \rfloor + q + 1$. 

Hence using the principle of Mathematical induction, we have $\mathbb{P}[N_k^{\pi^*}(\tb{\ti{s}}) \geq x-1]$ is same for all $\tb{\ti{s}} \in \mathcal{S}_{r+1}$.

Thus, going back to expression for $\mathbb{P}[N_k^{\pi^*}(\tb{\ti{s}}) \geq x]$ in Equation \eqref{eqn:prob_nxs}, $\mathbb{P}[N_k^{\pi^*}(\tb{\ti{s}}) \geq x-1]$ is also not dependent on $\tb{\ti{s}} \in \mathcal{S}_{r+1}$. Therefore, $\mathbb{P}[N_k^{\pi^*}(\tb{\ti{s}}) \geq x]$ is same for all $\tb{\ti{s}} \in \mathcal{S}_{r+1}$. We denote this as $\mathbb{P}[N_k^{\pi^*}(r+1) \geq x]$

Finally, we need to show that, 
\begin{align}
    \mathbb{P}[N_k^{\pi^*}(\tb{\ti{s}}) \geq x] \geq \mathbb{P}[N_k^{\pi^*}(\tb{\ti{s}}') \geq x], \quad \forall ~ \tb{\ti{s}}' \in \cup_{r' \in \{0\} \cup [r]}\mathcal{S}(r')
\end{align}

with equality at $\tb{\ti{s}}' = \tb{\ti{s}}$. Moreover, recall  for any $\tb{\ti{s}} \in \mathcal{S}_{r+1}$, we have
\begin{align}
    &\mathbb{P}[N_k^{\pi^*}(\tb{\ti{s}})\geq x] \nonumber
    \\
    &=   \mathbb{P}(\tb{\ti{s}}|\tb{\ti{s}},\pi^*(\tb{\ti{s}})) \mathbb{P}[N_k^{\pi^*}(\tb{\ti{s}}) \geq x-1] + \sum_{r'=1}^r \binom{r+1}{r'}  .  p^*_{r+1,r'}  \mathbb{P}[N_k^{\pi^*}(r') \geq x-1] 
    \\ 
    &= \mathbb{P}(\tb{\ti{s}}|\tb{\ti{s}},\pi^*(\tb{\ti{s}})) \mathbb{P}[N_k^{\pi^*}(\tb{\ti{s}}) \geq x-1] + \sum_{r' = 1}^{ \lfloor \frac{r+1}{2} \rfloor } \binom{r+1}{r'}  .  p^*_{r+1,r'}  \mathbb{P}[N_k^{\pi^*}(r')  \geq x-1]\nonumber
    \\
    & \quad + \sum_{r' = \lfloor \frac{r+1}{2} \rfloor +1}^{ r} \binom{r+1}{r'}  .  p^*_{r+1,r'}  \mathbb{P}[N_k^{\pi^*}(r') \geq x-1] 
\end{align}
In the above, we just split the summation. Below, we use Lemma \ref{claim:probability_inequality} with Equations \eqref{eqn:del1} and \eqref{eqn:del2} and simplify further by rearranging the summations, 
\begin{align}
    &\mathbb{P}[N_k^{\pi^*}(\tb{\ti{s}}) \geq x] \nonumber
    \\
    &= \mathbb{P}(\tb{\ti{s}}|\tb{\ti{s}},\pi^*(\tb{\ti{s}})) \cdot \mathbb{P}[N_k^{\pi^*}(\tb{\ti{s}}) \geq x-1] + \sum_{r'= 1}^{ \lfloor \frac{r+1}{2} \rfloor } \left( \binom{r}{r'}  .  p^*_{r,r'} - \delta_{r,r'} \right)  \mathbb{P}[N_k^{\pi^*}(r') \geq x-1] \nonumber
    \\
    &\quad + \sum_{r' = \lfloor \frac{r+1}{2} \rfloor +1}^{ r} \left( \binom{r}{r'}  .  p^*_{r,r'}+ \delta_{r,r'}  \right)\mathbb{P}[N_k^{\pi^*}(r') \geq x-1] 
    \\ 
    &= \mathbb{P}(\tb{\ti{s}}|\tb{\ti{s}},\pi^*(\tb{\ti{s}})) \cdot \mathbb{P}[N_k^{\pi^*}(\tb{\ti{s}}) \geq x-1] + \sum_{r' = 1}^{ \lfloor \frac{r+1}{2} \rfloor } \left(\binom{r}{r'}  .  p^*_{r,r'} . \mathbb{P}[N_k^{\pi^*} (r') \geq x-1]\right) \nonumber
    \\
    &\quad -  \sum_{r' = 1}^{\lfloor \frac{r+1}{2} \rfloor }\left(\delta_{r,r'} . \mathbb{P}[N_k^{\pi^*}(r') \geq x-1]\right)   + \sum_{r' = \lfloor \frac{r+1}{2} \rfloor +1}^{ r} \left(\binom{r}{r'}  .  p^*_{r,r'} . \mathbb{P}[N_k^{\pi^*}(r') \geq x-1]\right) \nonumber
    \\
    &\quad + \sum_{r' = \lfloor \frac{r+1}{2} \rfloor +1}^{r} \left(\delta_{r,r'} . \mathbb{P}[N_k^{\pi^*}(r') \geq x-1] \right)  
    \\ 
    &= \mathbb{P}(\tb{\ti{s}}|\tb{\ti{s}},\pi^*(\tb{\ti{s}})) \cdot  \mathbb{P}[N_k^{\pi^*}(\tb{\ti{s}}) \geq x-1] + \sum_{r' = 1}^{ r} \left( \binom{r}{r'}  .  p^*_{r,r'} . \mathbb{P}[N_k^{\pi^*}(r')  \geq x-1]\right) \nonumber
    \\
    &\quad -  \sum_{r' =1}^{ \lfloor \frac{r+1}{2} \rfloor}\left(\delta_{r,r'} . \mathbb{P}[N_k^{\pi^*}(r') \geq x-1] \right)   + \sum_{r' = \lfloor \frac{r+1}{2} \rfloor +1}^{ r} \left( \delta_{r,r'} . \mathbb{P}[N_k^{\pi^*}(r') \geq x-1] \right) 
    \\ 
    &= \mathbb{P}(\tb{\ti{s}}|\tb{\ti{s}},\pi^*(\tb{\ti{s}})) \cdot  \mathbb{P}[N_k^{\pi^*}(\tb{\ti{s}}) \geq x-1] + \mathbb{P}[N_k^{\pi^*}(r) \geq x]   \nonumber
    \\
    &\quad -  \sum_{r' = 1}^{ \lfloor \frac{r+1}{2} \rfloor }\left( \delta_{r,r'} . \mathbb{P}[N_k^{\pi^*}(r') \geq x-1] \right)  + \sum_{r'= \lfloor \frac{r+1}{2} \rfloor +1}^{r} \left(\delta_{r,r'} . \mathbb{P}[N_k^{\pi^*}(r')  \geq x-1]\right)   \label{eqn:psimp}
\end{align}
where in the last step we use the definition of $\mathbb{P}[N_k^{\pi^*}(r) \geq x]$.

Now, using the Induction assumption, we have for some $\Tilde{\tb{\ti{s}}} \in \mathcal{S}_r$ and any $x \in \mathbb{R}^+$ 
\begin{align}
    \mathbb{P}[N_k^{\pi^*}(\Tilde{\tb{\ti{s}}}) \geq x] = \mathbb{P}[N_k^{\pi^*}(r) \geq x] \geq \mathbb{P}[N_k^{\pi^*}(\Tilde{\tb{\ti{s}}}') \geq x]
\end{align}
for any $\Tilde{\tb{\ti{s}}}' \in \mathcal{S}(\Tilde{\tb{\ti{s}}})$. Taking $\Tilde{\tb{\ti{s}}}' \in \mathcal{S}_{r-1}(\tb{\ti{s}})$ and using the induction assumption further, we have
\begin{align}
    \mathbb{P}[N_k^{\pi^*}(\Tilde{\tb{\ti{s}}}) \geq x] = \mathbb{P}[N_k^{\pi^*}(r) \geq x] \geq \mathbb{P}[N_k^{\pi^*}(\Tilde{\tb{\ti{s}}}') \geq x] = \mathbb{P}[N^{\pi^*}_k(r-1) \geq x]
\end{align}

Using the same arguments as above recursively, we finally obtain
\begin{align}
    \mathbb{P}[N_k^{\pi^*}(r) \geq x] \geq \mathbb{P}[N^{\pi^*}_k(r-1) \geq x]  \geq \dots  \geq \mathbb{P}[N^{\pi^*}_k(1) \geq x] \geq \mathbb{P}[N^{\pi^*}_k(0) \geq x] = 0 \label{eqn:mon}
\end{align}
Note that the above is true for any $x \in \mathbb{R}^+$. 
Using the monotonicity relation above (replacing $x$ by $x-1$), we further simplify Equation \eqref{eqn:psimp} as below: 
\begin{align}
    &\mathbb{P}[N_k^{\pi^*}(\tb{\ti{s}})\geq x] \nonumber
    \\
    &\geq  \mathbb{P}(\tb{\ti{s}}|\tb{\ti{s}},\pi^*(\tb{\ti{s}})) \cdot  \mathbb{P}[N_k^{\pi^*}(\tb{\ti{s}}) \geq x-1]  -  \sum_{r'=1}^{ \lfloor \frac{r+1}{2} \rfloor } \left( \delta_{r,r'} \cdot \mathbb{P} \left[ N_k^{\pi^*} \left( \left\lfloor \frac{r+1}{2} \right\rfloor + 1 \right) \geq x-1 \right] \right) \nonumber
    \\
    &\quad + \mathbb{P}[N_k^{\pi^*}(r) \geq x] + \sum_{r' =\lfloor \frac{r+1}{2} \rfloor +1}^{r} \left(\delta_{r,r'} \cdot \mathbb{P} \left[ N_k^{\pi^*} \left( \left\lfloor \frac{r+1}{2} \right\rfloor + 1 \right) \geq x-1 \right] \right) 
    \\ 
    &=  \mathbb{P}(\tb{\ti{s}}|\tb{\ti{s}},\pi^*(\tb{\ti{s}})) \cdot \mathbb{P}[N_k^{\pi^*}(\tb{\ti{s}}) \geq x-1] + \mathbb{P}[N_k^{\pi^*}(r)  \geq x] \nonumber
    \\
    & \quad -  \left[ \sum_{r'= 1}^{ \lfloor \frac{r+1}{2} \rfloor }\delta_{r,r'} - \sum_{r'= \lfloor \frac{r+1}{2} \rfloor +1}^{r} \delta_{r,r'} \right] \cdot \mathbb{P} \left[ N_k^{\pi^*} \left( \left\lfloor \frac{r+1}{2} \right\rfloor + 1 \right) \geq x-1 \right]  
    \\ 
    & = \mathbb{P}(\tb{\ti{s}}|\tb{\ti{s}},\pi^*(\tb{\ti{s}})) \cdot \mathbb{P}[N_k^{\pi^*}(\tb{\ti{s}}) \geq x-1] + \mathbb{P}[N_k^{\pi^*}(r) \geq x] \nonumber
    \\
    & \quad -  \mathbb{P}(\tb{\ti{s}}|\tb{\ti{s}},\pi^*(\tb{\ti{s}})) \cdot  \mathbb{P} \left[ N_k^{\pi^*} \left( \left\lfloor \frac{r+1}{2} \right\rfloor + 1 \right) \geq x-1 \right]
    \\ 
    & > \mathbb{P}(\tb{\ti{s}}|\tb{\ti{s}},\pi^*(\tb{\ti{s}})) \mathbb{P}[N_k^{\pi^*}(\tb{\ti{s}}) \geq x-1] + \mathbb{P}[N_k^{\pi^*}(r) \geq x]    -  \mathbb{P}(\tb{\ti{s}}|\tb{\ti{s}},\pi^*(\tb{\ti{s}})) \cdot \mathbb{P}[N_k^{\pi^*}( r) \geq x-1] 
\end{align}
In the last second step, we use Equation \eqref{eqn:p_r_r}. For the last step, we further use the monotonicity result in Equation \eqref{eqn:mon} for $x-1$. Thus, we have
\begin{align}
    \mathbb{P}[N_k^{\pi^*}(\tb{\ti{s}}) \geq x] - \mathbb{P}[N_k^{\pi^*}(r) \geq x] \geq \mathbb{P}(\tb{\ti{s}}|\tb{\ti{s}},\pi^*(\tb{\ti{s}})).(\mathbb{P}[N_k^{\pi^*}(\tb{\ti{s}}) \geq x-1] - \mathbb{P}[N_k^{\pi^*}(r) \geq x-1])
\end{align}
By recursion and same arguments as before that follows Equation \eqref{eqn:pnxnx}  we have
\begin{align}
    \mathbb{P}[N_k^{\pi^*}(\tb{\ti{s}}) \geq x] = \mathbb{P}[N_k^{\pi^*}(r+1) \geq x] >  \mathbb{P}[N_k^{\pi^*}(r) \geq x]
\end{align}
Note that the equality above was already show earlier in the discussion following Equation \eqref{eqn:pneq}.
Hence the overall main induction argument for $r$ holds.     
\end{proof}
