# Supplementary material for: Regret Lower Bounds for Decentralized Multi-Agent Stochastic Shortest Path Problems
Source: arXiv:2511.04594 source file (2025-12-13)
Supplement: Supplementary file 3 [file notations.tex]

\paragraph{Notations and Definitions/Glossary.} 

$n$ represents the number of agents in the system. \\
$\mathcal{N} = [n] $ represents the set of agents. \\
$\mathcal{S}$ is the set of all (global) states and $\mathcal{A}$ is the set of all (global) actions. \\
Nodes are denoted as simple small case letters  i.e., $\{s,g\}$. \\
State, same as Global State, is represented as bold-face small case letter i.e., $\tb{\ti{s}} = \{s_1,s_2,\dots,s_n\}$ where for each $i \in [n]$, $s_i$ denotes the node at which agent $i$ is present. \\
Action, same as Global action, is denoted by bold-face small case letter i.e., $\tb{\ti{a}} = \{a_1,a_2,\dots,a_n\}$ where for any agent $i \in [n]$, $a_i$ denotes the individual action taken by agent $i$. \\
For our instances, individual actions $a_i$ are $(d-1)$ dimensional. The $j^{th}$ component of $a_i$ for any $j \in [d-1]$ is represented as $a_{i,j}$  for any $i \in [n].$ \\
For any $\tb{\ti{s}} \in \mathcal{S}$, $\mathcal{S}(\tb{\ti{s}})$ denotes the set of all states $\tb{\ti{s}}' \in \mathcal{S}$ that can be reached in the next step from $\tb{\ti{s}}$ with non-zero probability under some action $\tb{\ti{a}} \in \mathcal{A}$. \\
For any state $\tb{\ti{s}} \in \mathcal{S}$, let $r$ denote the number of agents located at the node $s$ when the global state is $\tb{\ti{s}}$. We refer to such a state $\tb{\ti{s}}$ as being of \emph{type} $r$. \\
For any $r \in [n] \cup \{0\}$, we represent the set of all states of \emph{type} $r$ as $\mathcal{S}_r$. \\
If the probability of reaching $\tb{\ti{s}}'$ in the next step by taking action $\tb{\ti{a}}$ at $\tb{\ti{s}}$ is non-zero, we say that \emph{$\tb{\ti{s}}'$ is reachable from $\tb{\ti{s}}$ under $\tb{\ti{a}}$}. If there exists some $\tb{\ti{a}} \in \mathcal{A}$ such that $\tb{\ti{s}}'$ is \emph{reachable from $\tb{\ti{s}}$ under $\tb{\ti{a}}$}, we say that \emph{$\tb{\ti{s}}'$ is reachable from $\tb{\ti{s}}$}. \\
Note that our instance construction ensures that if a transition $\tb{\ti{s}} \rightarrow \tb{\ti{s}}'$ occurs with non-zero probability under some action, then it occurs with non-zero probability under all actions, and vice versa. \\
For any $\tb{\ti{s}} \in \mathcal{S}$ of \emph{type} $r \in [n]$ and for any $r' \in [r] \cup \{0\}$, we define $\mathcal{S}_{r'}(\tb{\ti{s}})$ as the set of all states of \emph{type} $r'$ that are \emph{reachable} from $\tb{\ti{s}}$. \\
In the analysis of any valid state transition from $\tb{\ti{s}} $ of \emph{type} $r$ to $\tb{\ti{s}}'$ of \emph{type} $r'$, we have the following definitions: \\
In the state $\tb{\ti{s}}$, $\mathcal{I} = \{i_1,i_2,\dots,i_r\}$ denotes the set of all agents that are at node $s$ and $\mathcal{J} = \{j_1,j_2,\dots,j_{n-r}\}$ represents the set of all agents that are at node $g$. The set of all agents that transit from node $s$ to node $g$ during the transition from global state $\tb{\ti{s}}$ to $\tb{\ti{s}}'$ is represented as $ \{t_1,t_2,\dots,t_{r-r'}\} = \mathcal{T} \subseteq \mathcal{I}$. Further, we represent the set of agents that stay at node $s$ itself as $\mathcal{I} \cap \mathcal{T'}$. \\
For any $(\tb{\ti{s}}, \tb{\ti{a}},\tb{\ti{s}}') \in \mathcal{S} \times \mathcal{A} \times \mathcal{S}$, $\mathbb{P}(\tb{\ti{s}}'|\tb{\ti{s}}, \tb{\ti{a}})$ represents the probability that the next state is $\tb{\ti{s}}'$ given that action $\tb{\ti{a}}$ is taken at state $\tb{\ti{s}}$. \\
Any of our instances is defined by a fixed tuple $(n,\delta,\Delta, \theta)$ where $n \geq 1, \delta \in (2/5,1/2), \Delta<2^{-n}. \frac{1-2\delta}{1+n+n^2}$ and $\theta \in \Theta $ \\
Each $\theta$ is of the form $\theta = (\theta_1,1, \theta_2,1,\dots, \theta_n,1)$ where for every $i \in [n]$, $\theta_i \in \{\frac{-\Delta}{n(d-1)}, \frac{\Delta}{n(d-1)}\}^{d-1}$. The set of all such $\theta$'s is $\Theta$. \\
$\phi(\tb{\ti{s}}'|\tb{\ti{s}}, \tb{\ti{a}})$ is the feature associated with probability of transition from $\tb{\ti{s}} $ to $\tb{\ti{s}}'$ under $\tb{\ti{a}}$ in the linear mixture model. \\
Under the linear function approximation of transition probabilities, the transition probabilities are given as : $\mathbb{P}(\tb{\ti{s}}'|\tb{\ti{s}}, \tb{\ti{a}}) = \langle \phi(\tb{\ti{s}}'|\tb{\ti{s}}, \tb{\ti{a}
}), \theta\rangle$ \\
$\binom{x}{y}$ represents the binomial coefficient associated with number of ways to choose $y$ objects out of $x$ identical objects.\\
$sgn(\cdot)$ represents the signum function. Takes value +1 if the term inside parenthesis is positive and -1 if it is negative, else 0.\\
$Q^{\pi}(\tb{\ti{s}}, \tb{\ti{a}})$ represents the action value function under policy $\pi$ for any $(\tb{\ti{s}}, \tb{\ti{a}}) \in \mathcal{S} \times \mathcal{A}$.  \\
$V^*(\tb{\ti{s}})$ for any $\tb{\ti{s}} \in \mathcal{S}$ represents the optimal value of state $\tb{\ti{s}}$. \\
$\tb{\ti{s}}_{\init}$ is the state where any episode starts. Here, all agents are at node $s$. $\tb{\ti{g}} = goal$ is the state where every episode ends. Here, all agents are at node $g$.\\
$\mathbb{E}_{\pi,\theta}[R_k]$ denotes the expected cumulative regret in the $k^{th}$ episode for the instance defined by $\theta$ for the algorithm $\pi$. \\
$\mathbb{E}_{\pi,\theta}[R(K)]$ represents the expected cumulative regret over $K$ episodes for the instance defined by $\theta$ for the given algorithm $\pi$. \\
$N_k$ denotes the (random) number of time steps in episode $k$. \\
$N$ represents the (random) total number of time steps during the learning period of $K$ episodes. \\
Thus, $N = \sum_{k=1}^K N_k$.\\
\textcolor{red}{Verify again later}
$N_{i,j}(\theta)$ represents the number of time steps during learning instance $\theta$ that the $i^{th}$ agent takes a suboptimal action that differs from the optimal action at the $j^{th}$ index for any $i \in [n]$ and $j \in [d-1]$. \\
Analogously, quantities $N^-$ and $N^-_{i,j}(\theta)$ are defined for the capped learning process by truncating the sum to predefined time horizon length $T$. \\
$N^\pi_k(\tb{\ti{s}})$ denotes the (random) number of steps to reach $\tb{\ti{g}}$ by starting at $\tb{\ti{s}}$ and following $\pi$.  \\
For any $x \in \mathbb{R}^+$, deterministic algorithm $\pi$, $\tb{\ti{s}} \in \mathcal{S}$, $\mathbb{P}[N^\pi_k(\tb{\ti{s}}) \geq x]$ represents the probability that starting at $\tb{\ti{s}}$, following $\pi$, the number of time steps to reach $\tb{\ti{g}} =goal$ is greater than or equal to $x$.
