# Supplementary material for: Regret Lower Bounds for Decentralized Multi-Agent Stochastic Shortest Path Problems
Source: arXiv:2511.04594 source file (2025-12-13)
Supplement: Supplementary file 12 [file comments.tex]

Q. What is the class of decentralized algorith,s for which the provided bound holds?
A. All decentralized algorithms since we didn't make any assumptions on how much information is allowed to be shared. Hence, the same bound also hold for centralized algorithms.

Q. Theta parameter set is finite?
A. For fixed n, d its cardinality is $2^(n(d-1))$. To clear, it is parameter of instance and not of policy hence there is no moving along gradient kind of idea.

Q. Why the single agent lower bound not enough for multi-agent?
A. The single agent lower bound given earlier is for 2 state system. In multiple agent case, even with central controller, we cannot escape $2^n$ states. The earlier results need to be extended for this settings.

C. There is definitely a one to one mapping from decentralised problem to centralised problem 

Q. To modify statement in the report : valid lower-bound...
A. I don't think there's ambiguity: i don't mean "all" know upper bounds in that statement. If someone can show that (any) lower bound for MASSP exceeds any (even a single) single agent SSP upper bound, then MASSP is harder.
