# Supplementary material for: Regret Lower Bounds for Decentralized Multi-Agent Stochastic Shortest Path Problems
Source: arXiv:2511.04594 source file (2025-12-13)
Supplement: Supplementary file 15 [file cor3.tex]

\subsection{Proof of Corollary \ref{corollary:pn_x}}

% \pt{Now this is the corollary of Lemma 8. So, if}

\textbf{Recall the Corollary \ref{corollary:pn_x}.}
\textit{An immediate corollary of the above lemma is that $\mathbb{P}[N_k^{\pi^*}(r) \geq x]$ is ordered for any $x \in R^+$ i.e., $\mathbb{P}[N_k^{\pi^*}(n) \geq x] \geq \mathbb{P}[N_k^{\pi^*}(n-1) \geq x] \geq \cdots \geq \mathbb{P}[N_k^{\pi^*}(2)  \geq x]\geq \mathbb{P}[N_k^{\pi^*}(1)  \geq x]\geq \mathbb{P}[N_k^{\pi^*}(0) \geq x] =0 $}

From Lemma $\ref{lemma:episodelength}$, taking $\tb{\ti{s}} = \tb{\ti{s}}_{\init}$ and some $\tb{\ti{s}}' \in \mathcal{S}(n-1)$,
\begin{align}
    \mathbb{P}[N_k^{\pi^*}(\tb{\ti{s}}_{\init}) \geq x]  = \mathbb{P}[N_k^{\pi^*}(n) \geq x]  \geq \mathbb{P}[N_k^{\pi^*}(n-1) \geq x]
\end{align}
By recursion, the corollary follows.
